# Supplementary material for: From Merging Frameworks to Merging Stars: Experiences using HPX, Kokkos and SIMD Types
Source: arXiv:2210.06439 source file (2023-05-09)
Supplement: Supplementary file 1 [file espm2_ad_appendix_rc3.pdf]

## APPENDIX A

### ARTIFACT DESCRIPTION APPENDIX: FROM MERGING FRAMEWORKS TO MERGING STARS: EXPERIENCES USING HPX, KOKKOS AND SIMD TYPES

#### A. Abstract

Octo-Tiger, a large-scale 3D AMR code for the merger of stars, uses a combination of HPX, Kokkos and explicit SIMD types, aiming to achieve performance-portability for a broad range of heterogeneous hardware. However, on A64Fx CPUs, we encountered several missing pieces, hindering performance by causing problems with the SIMD vectorization. Consequently, we add `std::experimental::simd` as an option to use in Octo-Tiger’s Kokkos kernels alongside Kokkos SIMD, and further add a new SVE backend. Additionally, we amend missing SIMD implementations in the Kokkos kernels within Octo-Tiger’s hydro solver. We test our changes by running Octo-Tiger on three different CPUs: A A64Fx, and recent Intel Icelake and AMD Epyc CPUs, evaluating SIMD speedup and node-level performance. Using our changes, we get a good SIMD speedup on the A64Fx CPU, as well as noticeable speedups on the other two CPU platforms. However, we also experience a scaling issue on the Epyc CPU.

#### B. Description

##### 1) Check-list (artifact meta information):

- **Algorithm:** Octo-Tiger primarily uses the Fast-Multipole Method for the gravity solver and finite volumes for the hydro solver
- **Program:** Octo-Tiger
- **Compilation:** g++11.2
- **Hardware:** Intel CPU, AMD CPU, A64Fx CPU
- **Output:** Python Script to re-run the plots is available
- **Experiment workflow:** Iterate over cores and SIMD extensions, Bash scripts to re-run experimentation are available
- **Experiment customization:** Modified Kokkos and Octo-Tiger, commits and patches are available
- **Publicly available?:** GitHub

##### 2) How software can be obtained (if available):

Octo-Tiger can be obtained on GitHub: <https://github.com/STELLAR-GROUP/octotiger>

We used two Octo-Tiger commits:

- 2461163996c576a5d43b4cd1a7f8c295d446f925 (for using more tasks in the multipole kernels to generate Figure 5.)
- 9437e172264a4c7b3f24ec4ccd4c380feba26755 (for all other tests)

3) *Hardware dependencies:* We run our tests on three different machines:

- 1) One A64Fx node on Ookami.
- 2) One university server (at LSU) containing a two-socket Intel® Xeon® Platinum 8358 Processor CPU (64 cores)
- 3) One university server (at LSU) containing a two-socket AMD Epyc 7H12 (128 cores)

Memory requirements for the scenarios we use are minimal and should not exceed 4 GB for each scenario itself.

4) *Software dependencies:* Octo-Tiger has multiple, mandatory software dependencies:

- HPX: 1.8.0
- Kokkos: 2640cf70de338618a7e4fe10590b06bc1c239f4c (on Intel and AMD), 596bb0b1b (on Ookami)
- HPX-Kokkos: 20a44967c742f5a7670b4dff9658d9973bf849f2 (<https://github.com/STELLAR-GROUP/hpx-kokkos>)
- CPPuddle: 6127562897dc2940869d744d490d0eb7b6fa37bc (<https://github.com/SC-SGS/Cppuddle>)
- Vc: 1.4.1
- Jemalloc: 5.2.1
- silo: 4.10.2
- HDF5: 1.8.12
- Boost: 1.75 (on Intel and AMD machine), 1.78 (on Ookami)
- SVE type library: e3b2fb8d7bfda5d6eda90efee29fafdcbe895a25 (<https://github.com/srinivasyadav18/sve>)

All dependencies are available online! We have added links for the lesser known ones though, to ease reproducibility.

For ease of use there are buildscripts available: <https://github.com/STELLAR-GROUP/OctoTigerBuildChain>

Kokkos has been customized based on the commits specified here, to allow the single-task optimization mentioned in section V A). This has not yet been upstreamed. However, the buildscripts contain the patchfile for this (kokkos-single-task.patch) and apply the patch automatically during building.

5) *Datasets:* No additional datasets are required! The inputfile required for the “rotating star” scenario can be created using the binary `gen_rotating_star_init` which will be built automatically when building Octo-Tiger. The configuration files `blast.ini` and `rotating_star.ini` are also part of the Octo-Tiger repository (in the `test_problems` sub directory).

Using these configuration files, the Rotating Star scenario can be started with these parameters (adapt path to the ini files):

Parameters: `--config_file=rotating_star.ini`  
`--unigrid=1 --max_level=3 --stop_step=10`  
`--correct_am_hydro=0 --theta=0.34`  
`--disable_output=1`

For the Sedov Blast Wave scenario:

Parameters: `--config_file=blast.ini`  
`--unigrid=1 --max_level=3 --stop_step=10`  
`--correct_am_hydro=0 --disable_output=1`

Additional parameters steer whether the KOKKOS or LEGACY kernels are used:

- `--hydro_host_kernel_type=KOKKOS`
- `--multipole_host_kernel_type=KOKKOS`
- `--monopole_host_kernel_type=KOKKOS`

#### C. Installation

There are buildscripts available to ease to building of Octo-Tiger with the given software dependencies above: <https://github.com/STELLAR-GROUP/OctoTigerBuildChain>

1) *Intel Node:* To install on the LSU Intel machine, use the buildscripts commit: `f945f3184e030d60d619fbe69a63a449024e6e53`

Make sure modules `gcc/11.2.1` and `hwloc 2.4.1` are loaded!

Within the root directory of the buildscripts, run:

```
./build-all.sh Release with-CC without-cuda without-mpi
without-papi with-apex with-kokkos with-simd with-hpx-
backend-multipole with-hpx-backend-monopole with-hpx-
cuda-polling without-otf2 boost hdf5 silo jemalloc vc hpx
kokkos cppuddle octotiger
```

2) *AMD Node*: To install on LSU AMD machine, use the buildscripts commit: `49a7224f5ba951d8c51de3af14b9b2f5d6f50689`

Make sure modules gcc/11.2.1 and hwloc 2.4.1 are loaded!

Within the root directory of the buildscripts, run:

```
./build-all.sh Release with-CC without-cuda without-mpi
without-papi with-apex with-kokkos with-simd with-hpx-
backend-multipole with-hpx-backend-monopole with-hpx-
cuda-polling without-otf2 boost hdf5 silo jemalloc vc hpx
kokkos cppuddle octotiger
```

3) *Ookami A64Fx Node*: To install on LSU AMD machine, use the buildscripts commit: `d095bbedc06ae489521ed42a7ab2891d582a1546`

To install on Ookami, use the buildscripts commit: Make sure the module gcc/11.2.0 cmake/3.22.1 and hwloc/2.4.1 are loaded

Within the root directory of the buildscripts, run:

```
./build-all.sh Release with-CC without-cuda without-mpi
without-papi with-apex with-kokkos with-simd with-hpx-
backend-multipole with-hpx-backend-monopole with-hpx-
cuda-polling without-otf2 boost hdf5 silo jemalloc vc hpx
kokkos cppuddle octotiger
```

4) *Changing the SIMD types*: To switch SIMD types and libraries manually, the Octo-Tiger CMAKE flags can be used (modify build-octotiger.sh in the buildscripts):

- OCTOTIGER\_KOKKOS\_SIMD\_LIBRARY
- OCTOTIGER\_KOKKOS\_SIMD\_EXTENSION

The experiment bash scripts will do this automatically!

#### D. Experiment workflow

The scripts to perform the experiments on the Intel and AMD node can be found on GitHub: <https://github.com/G-071/octotiger-performance-tests/tree/master/rostand/node-level-scaling-tests>

The experiment `test_cpu_performance.sh` gathers all the runtime data when being launched after building within the root directory of the buildscripts.

The experiment itself iterates over all core and SIMD configurations, generating a log file containing the runtime data for the application and the compute kernels in csv format.

There are multiple scenario files within the GitHub repository available. To make the experiment work, you need to pass one (of the rotating star ones) to the script. The scenario files mostly contain the core configuration and specify the SIMD types to be used on each machine.

The bash script `test_cpu_performance.sh` for experiment needs to be run from the root directory of the buildscripts. Afterwards run the second bash script `test_hydro_speedup.sh`, also within the buildscripts root directory, to obtain the runtime data for the last figure in the paper.

Due to a change in the output format, the tests for Ookami can be found also on GitHub but in a different directory: <https://github.com/G-071/octotiger-performance-tests/tree/master/ookami/node-level-scaling-tests> However, the process of running the tests is the same as for the Intel and AMD node otherwise.

#### E. Evaluation and expected result

To evaluate the data, there is a `plot_node_level_scaling.py` file available <https://github.com/G-071/octotiger-performance-tests/tree/master/rostand/node-level-scaling-tests/plot> which can be used to plot the data obtained on each machine to generate the graphs in the paper! One needs to pass the file containing the csv results from the machines via `--filename=` (see `test_cpu_performance.sh`) in addition to the utilized SIMD extension `--simd_key`, for example AVX512. The python script expects pandas, numpy and matplotlib to be available. This should plot the node-level scaling graphs and the SIMD speedup graphs and immediately store them as PDFs in the same directory. To plot the last figure, the script also expects the other results, obtained by running `test_hydro_speedup.sh` test, to be present in the files:

- icelake\_legacy\_test.data
- epyc\_legacy\_test.data
- arm\_legacy\_test.data

The expected results are plots similar to what is shown in the paper!

#### F. Experiment customization

Kokkos gets modified with a patch as outlined above. To generate Figure 5, at different Octo-Tiger commit (see above) has to be used before running the experiment script!
